# Supplementary material for: Hybrid-State Free Precession in Nuclear Magnetic Resonance
Source: arXiv:1807.03424 ancillary file (2018-07-09)
Supplement: Supplementary file 1 [file HSFP_Paper_Supporting_Material.pdf]

# Supporting Material for: Hybrid-State Free Precession in Nuclear Magnetic Resonance

## A. IR-bSSFP as a Special Case of IR-bHSFP

In the following, we will assume a constant $\vartheta$, which converts a IR-bHSFP to a standard IR-bSSFP experiment[1] and allows us to solve the integrals in Eq. (7):

$$r(t) = \exp\left(-t/T_1^*\right) \cdot \left( r_0 - \frac{\cos\vartheta}{\frac{T_1}{T_2} \cdot \sin^2\vartheta + \cos^2\vartheta} \right) + \frac{\cos\vartheta}{\frac{T_1}{T_2} \cdot \sin^2\vartheta + \cos^2\vartheta} \tag{S1}$$

with

$$\frac{1}{T_1^*} = \frac{\sin^2\vartheta}{T_2} + \frac{\cos^2\vartheta}{T_1}. \tag{S2}$$

Transforming back to Cartesian coordinates with $S(t) = r(t) \cdot \sin\vartheta$, the signal is given by

$$S(t) = \exp\left(-t/T_1^*\right) \cdot \left(S_0 - S_{stst}\right) + S_{stst} \tag{S3}$$

with the initial signal $S_0 = r_0 \cdot \sin\vartheta$ (with $r_0 = -1$ for an inversion recovery experiment). The steady state signal is given by

$$S_{stst} = \frac{\sin\alpha}{\left(\frac{T_1}{T_2} + 1\right) - \cos\alpha \left(\frac{T_1}{T_2} - 1\right)} \tag{S4}$$

with the flip angle $\alpha = 2\vartheta$. The trigonometric identities $\sin(2\vartheta) = 2\sin\vartheta\cos\vartheta$ and $\cos(2\vartheta) = \cos^2\vartheta - \sin^2\vartheta$ were used for this transformation. Derived Eqs. (S2), (S3) and (S4) describe an exponential decay and are equivalent to Eqs. (2), (6) and (5) in Ref.[1]. Further, $1/T_1^*$ is equivalent to $R_{||}$ in Ref.[2] when assuming on-resonance ($\phi = \pi$).

## B. Relation to the Pseudo-Steady State

Ref.[3] names three conditions under which the spin-echo nature of bSSFP experiments[4] is maintained when varying the flip angle. The first of these *pseudo-SSFP conditions* effectively limits $\Delta\alpha$, and the hybrid-state adiabaticity condition is the stricter limit. The other two pseudo-SSFP conditions define a specific $T_R$-pattern to ensure the correct timing for the spin echo formation. The strict limitation of $\Delta\alpha$ and $\Delta\phi$ in the hybrid-state framework allow to approximate these pseudo-SSFP conditions by a constant $T_R$, such that hybrid-state experiments are a sub-set of pseudo-SSFP experiments.

The stricter conditions of the hybrid state also result in a more benign magnetization response. While the hybrid state eliminates the perpendicular component, the pseudo-SSFP approach strives to control it. As a result, the spectral response of pseudo-SSFP experiments is smooth only in the neighborhood of the on-resonant spin isochromat[3]. With increasing off-resonance, this property starts to fail, which makes the signal at those frequencies sensitive to inhomogeneous broadening. In contrast, the hybrid-state maintains this property at all Larmor frequencies.

## C. The Cramér-Rao Bound in Parameter Space

In the main article, the *rCRB* was analyzed only at the specific relaxation times used during the optimization. Fig. S1 analyzes the experiments that were optimized for $T_1 = 781$ ms and $T_2 = 65$ ms in a larger parameter space, i.e. over a larger range of $T_1$ and $T_2$

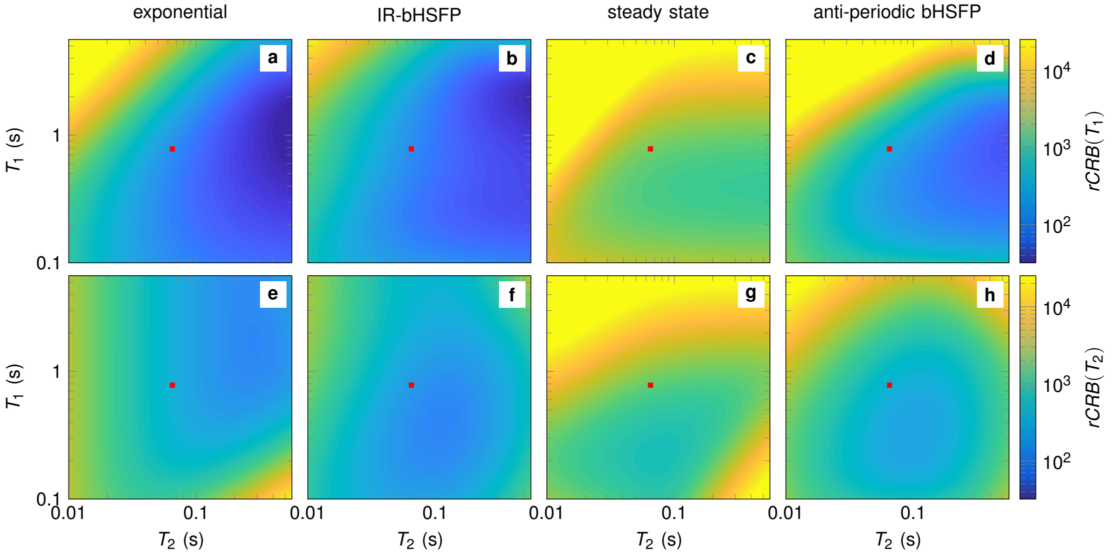


Supporting Figure S1: The performance of the optimized experiments is illustrated through plots of the relative Cramér-Rao bounds, which provide a lower bound for the noise in the retrieved relaxation times. All patterns were optimized for $T_1 = 781$ ms and $T_2 = 65$ ms, as indicated by the red square, and were tested for the entire parameter space in a sample MRF dictionary. The experiments have a $T_C = 3.8$s (cf. the black line Fig. 3). Note the logarithmic scale in all three dimensions.

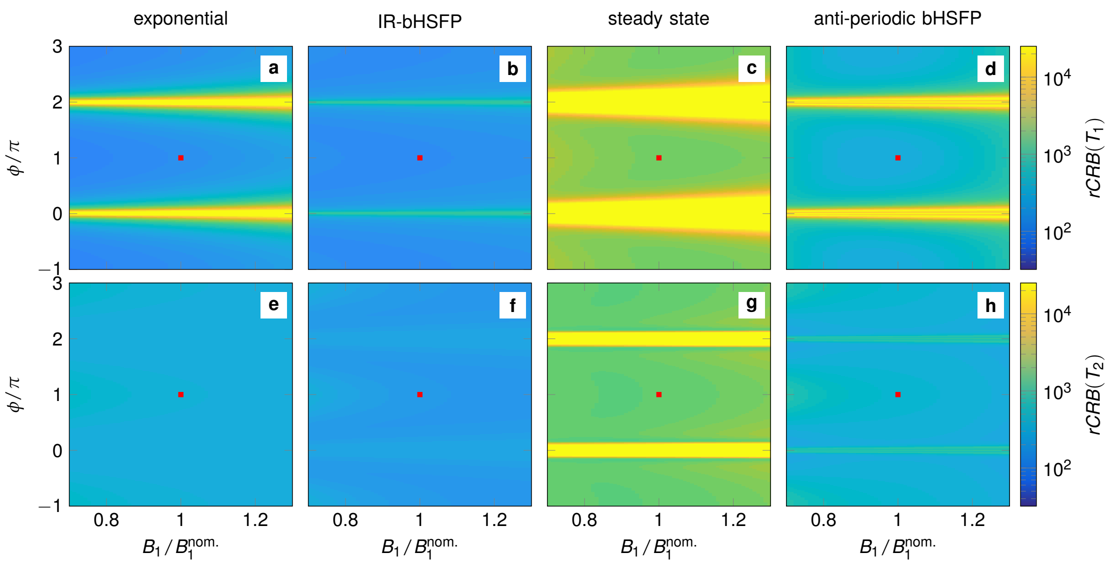


Supporting Figure S2: The performance of the optimized experiments is illustrated as a function of the main magnetic field, which is parameterized by the phase $\phi$, and of the inhomogeneities of the magnetic field $B_1$, which is used for spin excitation. The relaxation times were fixed to $T_1 = 781$ ms and $T_2 = 65$ ms, which are the values used during the optimization. The experiments have a $T_C = 3.8$s (cf. the black line Fig. 3). The red square indicates the nominal values.

values. The analyzed experiments were simultaneously optimized for $T_1$ and $T_2$. In this analysis, however, we examine $rCRB(T_1)$ and $rCRB(T_2)$ separately. Note that the relative Cramér-Rao bounds, as defined in Eqs. (35) and (36), take the correlation between the different parameters into account.

Fig. S1 confirms the improved encoding power of the hybrid state in comparison to exponential decay curves and the steady state (cf. Fig. 3). Especially the $rCRB(T_2)$ is reduced when using the IR-bHSFP experiment instead of the exponential one, but also the $rCRB(T_1)$ is improved for long $T_1$ and short $T_2$ (top left corner in Fig. S1b vs. a). A similar observation can be made when comparing the steady-state experiment to the anti-periodic hybrid-state one. In most of the areas of the $T_1$-$T_2$-space, the *rCRB* of the hybrid state is superior.

### D. $B_0$- and $B_1$-inhomogeneities

Spatial variations of the main magnetic field ($B_0$) are an inevitable problem in NMR, especially in MRI. In the present framework, they are captured by $\phi$ and affect the spin dynamics as detailed in Eqs. (5)-(7). The radio-frequency field used for spin excitation ($B_1$) is also subject to variations. In general, $B_1$ inhomogeneities scale the flip angle of RF pulses linearly and cause variations of the polar angle (Eq. (5)) and consequently of $r$, as described by Eq. (7).

The experiments' encoding power for $T_1$ and $T_2$ is analyzed in Fig. S2 for different $B_0$- and $B_1$-values under the assumption that the $B_0$ and $B_1$ variations are known from a separate measurement. Hardly any variation of the *rCRB* can be observed for any of the experiments within the analyzed range of parameters, apart from the vicinity of the stop-band ($|\sin\phi| \ll 1$). In the latter case, the magnetization lives close to the $x$-$y$-plane ($\vartheta \approx \pi/2$) for any $\sin^2\alpha \gg \delta$ (Eq. (5)), such that the magnetization is almost brought to naught (Eq. (7); Fig. S4). Intuitively, this leads a poor encoding of the parameters. In the case of the optimized steady-state experiment, the affected frequency band is larger compared to the hybrid-state experiments, in particular for $T_1$ (Fig. S2c vs. d). $B_1$-inhomogeneities seem to have a minor impact on the $T_1$ encoding capabilities with the biggest degradation observed in the anti-periodic hybrid-state experiment. Note that Figs. S2d,h do reflect the imperfection of the inversion pulse (Eq. (34)). For $T_2$, the effect of the $B_1$ inhomogeneities is slightly larger and the worst $rCRB(T_2)$ in all experiments is located at small $B_1$ values and an improvement of the *rCRB* compared to $B_1/B_1^{\text{nom.}} = 1$ can be observed at high $B_1$-values, reflecting the limit $\vartheta \leq \pi/4$, which was used during the optimization process and is exceeded for $B_1/B_1^{\text{nom.}} > 1$.

### E. Spin Dynamics

For comparison, the original MRF[5] pattern is depicted in Fig. S3a-c and represents a heuristic guess in the fully-transient state. Note that we depict here only the central isochromat and the dynamics of the other isochromats vary strongly. The original pseudo-SSFP (pSSFP) pattern[3] is a heuristic guess that approximates the hybrid state (cf. Section "Relation to the Pseudo-Steady State"), but inherits some fluctuations from the original MRF experiment (Fig. S3d-f).

The inversion recovery (IR) bSSFP experiments is a special case of the hybrid state, which forces the magnetization onto a straight line that goes from the southern half of the unit-sphere to the steady-state ellipse (Fig. S3g). The depicted experiment was optimized by a

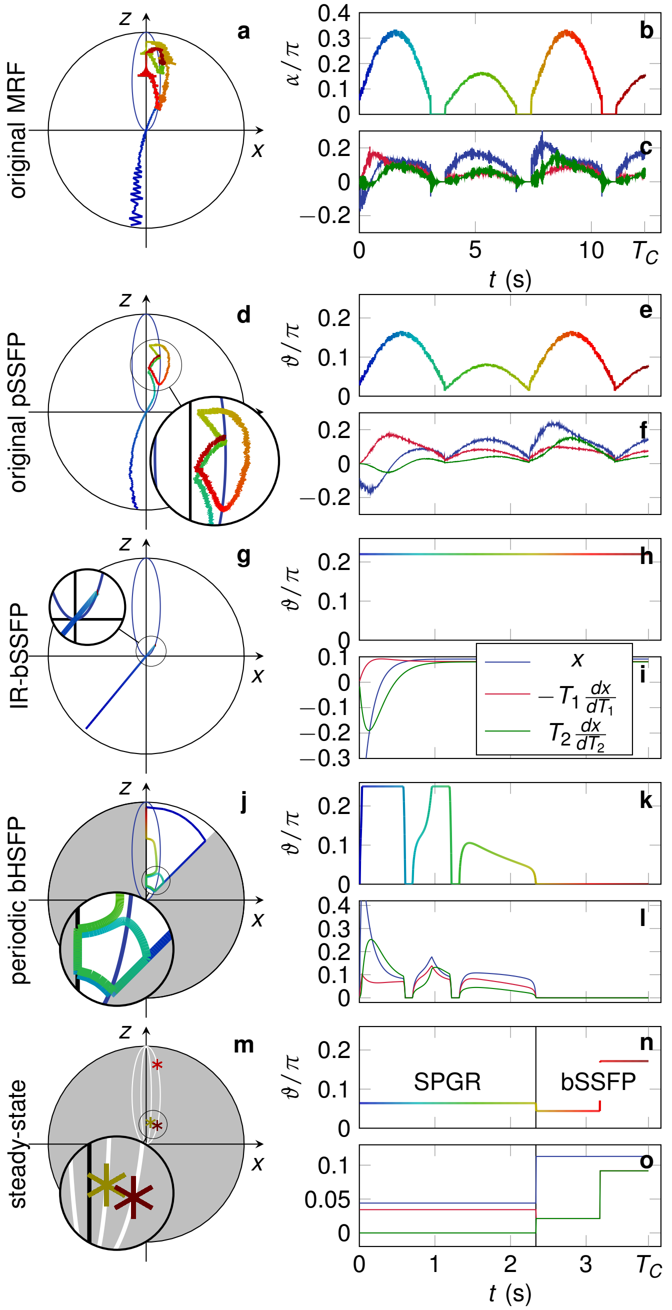


Supporting Figure S3: The spin dynamics is depicted for various experiments on Bloch spheres (**a**,**d**,**g**,**j**,**m**). The color scale of the $\vartheta$-pattern provides a reference for the trajectories on the Bloch spheres. The transversal magnetization and its normalized derivatives with respect to the relaxation times are the foundation of computing the relative Cramér-Rao bound and are shown in (**c**,**f**,**i**,**l**,**o**). The original MRF and pSSFP pattern represent heuristic guesses, while the other three experiments were jointly optimized for $T_1$ and $T_2$. Note that the $\vartheta$ of the bSSFP segment in (**j**-**l**) were retrospectively sorted in increasing order.

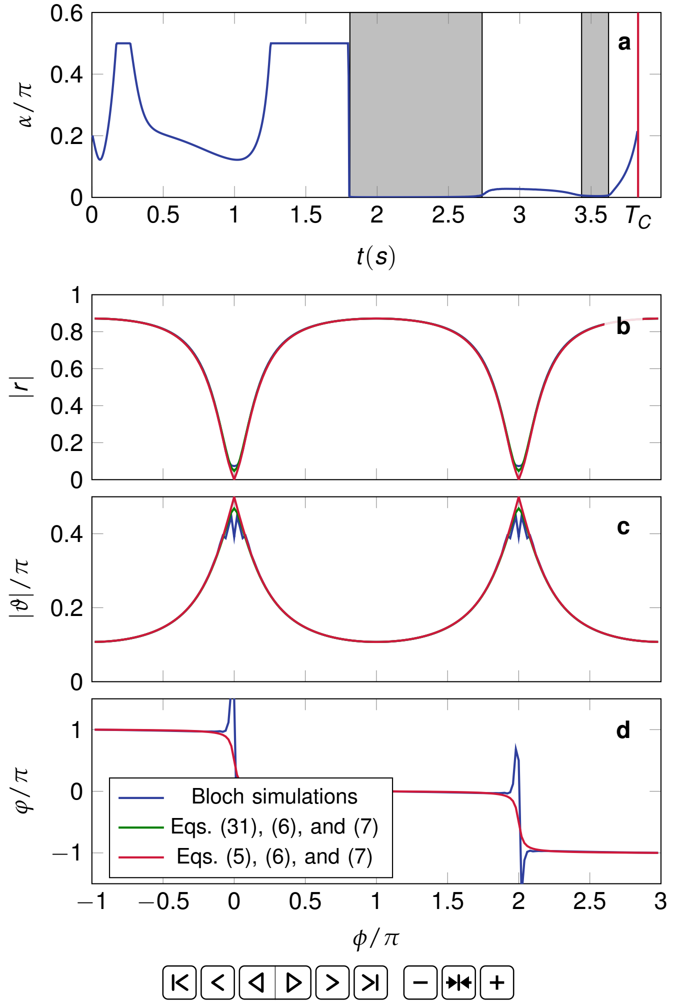


Supporting Figure S4: The derived Eqs. (5)-(7) are verified against Bloch simulations (Eq. (1)) at the example of the optimized anti-periodic pattern. Additionally, Eq. (31) provides the exact solution of $\vartheta$ in steady state. In agreement with the approximate nature of the derivation, good accordance can be observed anywhere apart from the vicinity of the stop band, which is defined by $|\sin \phi| \ll 1$. The gray areas indicate time points that were not acquired in the in vivo scan since the polar angle is close to zero, which violates assumptions made in the derivation and results in negligible signal. This figure assumes $\phi_{T_E} = \pi/2$, which is commonly achieved by setting $T_E = T_R/2$ in experiments with balanced gradient moments. *In order to run the animation, please use a PDF-viewer capable of JavaScript, such as the Adobe Acrobat Reader.*

global search for the constant $\vartheta$ with the lowest relative Cramér-Rao bound.

Fig. S3j-l show a hybrid-state experiment with periodic boundary conditions, which was optimized using the limit $0 \leq \vartheta \leq \pi/4$ for practical reasons. This effectively forces the magnetization to stay on the northern hemisphere, and the optimized trajectory splits into three segments: Starting from large $z$-values, the magnetization is excited to large $\vartheta$-values, where the spin dynamics is dominated by $T_2$-relaxation. Thereafter, the magnetization follows a small loop close to the origin, which combines $T_1$- and $T_2$-encoding. In the last segment, the magnetization stays close to the $z$-axis, where the dynamics is dominated by $T_1$-relaxation, before the cycle starts over again. The periodic boundary condition enforces $r(0) = r(T_C)$. The

optimizations also result in $\vartheta(0) \approx \vartheta(T_C)$, which is not enforced, but rather reflects the apparent optimality of smooth RF-pattern and ensures adherence to Eq. (3), similarly to the anti-periodic pattern (Fig. 4d,e).

The steady-state experiment depicted in Fig. S3m-o was optimized with an unbound polar angle. However, the steady-state model limits the search to the steady-state ellipse. As demonstrated by Eq. (S4), the steady-state signal of bSSFP experiments depends only on the ratio $T_1 / T_2$. In order to disentangle $T_1$ and $T_2$, one commonly combines the bSSFP experiment with a gradient- and RF-spoiled gradient echo (SPGR) segment, whose steady-state magnetization does not depend on $T_2$[6]. The steady-state magnetization of the SPGR experiment lies on a different ellipse that depends on $T_R$ and $T_1$ (inner ellipse in Fig. S3m). Optimizations based on the steady-state model results in three discreet polar angles, one in the SPGR segment and two in the bSSFP segment (Fig. S3n). The polar angles in the bSSFP segment have the same signal intensity (Fig. S3o), which was already found to be optimal in literature[6]. Different from literature is, however, the single flip angle in the SPGR segment. In Ref.[6], the signal from two SPGR flip angles was utilized to quantify $T_1$ independent of the bSSFP segment. Accounting for the bSSFP segment in the $T_1$ quantification, the numerical optimization results in a single flip angle for all time points in the SPGR experiment, or in total in three different flip angles for disentangling three parameters ($T_1$, $T_2$ and proton density). Note that the $T_2'$-decay in the SPGR segment is neglected here.

### F. Spectral Response

Eq. (5) provides a variety of combinations of $\phi$ and $\alpha$ that result in the desired $\vartheta$-pattern. Throughout this paper, we set $\phi = \pi$ for the central Larmor frequency, which requires $\alpha = 2\vartheta$ for all hybrid-state experiments and the bSSFP segment of the steady-state experiment, while $\alpha = \vartheta$ correctly describes the SPGR segment. Fig. S4 verifies Eqs. (5)-(7) for anti-periodic boundary conditions by depicting the spectral response of the magnetization. Good accordance can be observed between the hybrid-state model and the Bloch simulations apart from the vicinity of the stop-band ($|\sin\phi| \ll 1$), which is in agreement with the approximations made in the derivation. In general, the depicted spectral response is smooth and the phase is almost constant within each pass band, which connects the absence of inhomogeneous broadening to the spin-echo-like behavior known for bSSFP experiments[3,4]. One can observe some fluctuations of $\vartheta$ and $\varphi$ in the Bloch simulation around the time of the zero-crossing ($t \approx 0.3$s), i.e. when $r \approx 0$. Note that these errors are negligible in Cartesian coordinates due to the small absolute value of the magnetization.

One can further observe how the hybrid-state model breaks down in the gray segments in Fig. S4. The rapid decrease in the flip angle at the beginning of the first gray segment violates the adiabaticity condition (Eq. (3)) so that we observe significant contributions of the orthogonal eigenstates. However, the expected hybrid-state signal is small because these segments fulfill $\vartheta \ll 1$. Consequently, we can simply discard the signal measured in these segments and by the end of the gray segment the population of the orthogonal eigenstates is sufficiently decayed. Note that the phase $\varphi$ is not well defined for $\vartheta \approx 0$, causing strong fluctuations of the phase at small polar angles. The condition $\alpha^2 \ll \delta$ is not fulfilled in the gray segments in Fig. S4, which was required for the eigenvector analysis[2]. Nevertheless, after the initial decay in the first gray segment, and throughout the second gray segment, we observe a residual error mostly in the vicinity of the stop band. The combination of a small $\alpha$ and a small $\phi$ results in a non-negligible factor $\xi$ in Eq. (32), making Eq. (5) invalid. However, using the exact solution of the steady-state $\vartheta$ (Eq. (31)) substantially mitigates these errors (green graphs in Fig. S4).

### G. In Vivo Experiments

Fig. S5 supplements Fig. 5 and shows all slices of the 3D dataset, acquired with the anti-periodic bHSFP experiment.

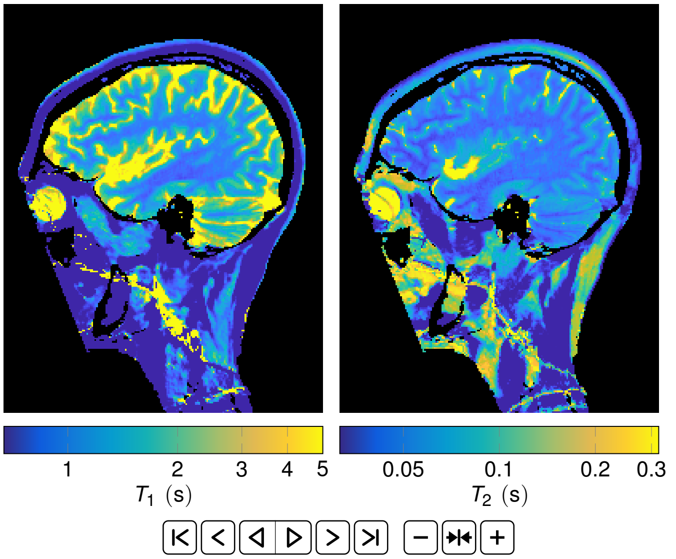


Supporting Figure S5: In order to supplement Fig. 5, all slices of the in vivo 3D data set are depicted. The data were acquired with the anti-periodic HSFP experiment depicted in Fig. 4e and fitted with the hybrid-state model (Eqs. (5) and (7)). The parameter maps have a resolution of 1 mm $\times$ 1 mm $\times$ 2 mm. Note the logarithmic scale of the $T_1$ and $T_2$ color map. The face was cut off in order to protect the volunteer's identity. *In order to run the animation, please use a PDF-viewer capable of JavaScript, such as the Adobe Acrobat Reader.*

### H. Population of the Orthogonal Eigenstate with Arbitrary Parameter Variations

In this section, we demonstrate that only small variations of $\alpha$ and $\phi$ result in a negligible perpendicular transient eigenstate. For simplicity, we focus on a zeroth order

approximation, i.e. we assume $\delta = 0$, or $E_1 = E_2$. This allows us to derive an explicit notation of the eigenvectors with perturbation theory in the same way it is done in Ref.[2]:

$$\mathbf{v}_S = \frac{1}{2\eta\sqrt{2(4\eta^2 + \cos\alpha - 1)}} \begin{pmatrix} 0 \\ -2\sin\frac{\phi}{2}\sin\alpha \\ (1+\cos\alpha)(1-\cos\phi) \\ 4\eta^2 \end{pmatrix}, \tag{S5}$$

$$\mathbf{v}_\parallel = \frac{1}{\eta} \begin{pmatrix} 0 \\ -\sin\frac{\alpha}{2} \\ \cos\frac{\alpha}{2}\sin\frac{\phi}{2} \\ 0 \end{pmatrix} \tag{S6}$$

and

$$\mathbf{v}_\perp^{(*)} = \frac{1}{\sqrt{2}\eta} \begin{pmatrix} \pm i\eta \\ \cos\frac{\alpha}{2}\sin\frac{\phi}{2} \\ \sin\frac{\alpha}{2} \\ 0 \end{pmatrix}. \tag{S7}$$

The approximation of the steady-state eigenvector is valid for $0 \neq 1 - E_1 \ll 1$, while the approximation of the perpendicular eigenvector requires $\cos\frac{\phi}{2} \neq 0$. In the case of $\cos\frac{\phi}{2} = 0$, the perpendicular eigenvectors become real valued (not shown here). The combination of those vectors compose the matrix $\mathbf{V} = (\mathbf{v}_S, \mathbf{v}_\parallel, \mathbf{v}_\perp, \mathbf{v}_\perp^*)$.

We now examine the matrix element $\mathbf{P}(\Delta\alpha, \alpha, \phi) = \mathbf{V}(\alpha + \Delta\alpha, \phi)^{-1}\mathbf{V}(\alpha, \phi)$ that describes the transfer from a steady state (with the parameters $\alpha$ and $\phi$) to the orthogonal transient eigenstate. If we assume that flip angle is changed by $\Delta\alpha$ and utilize Eqs. (S5) and (S7), we arrive at

$$P_{S\to\perp} = \frac{2\cos\frac{\alpha}{2}\cdot\sin\frac{\Delta\alpha}{2}\cdot(1-\cos\phi)\left(1 - \frac{1}{2}(\cos\phi + 1)(1 + (2\cos\frac{\alpha}{2}\cos^2\frac{\Delta\alpha}{2} - \cos\frac{\Delta\alpha}{2} - \cos\frac{\alpha}{2})(\cos\frac{\alpha}{2} + \cos\frac{\Delta\alpha}{2}))\right)}{\sqrt{(1-\cos^2\frac{\alpha}{2}\cos^2\frac{\phi}{2})(1-\cos^2\frac{\phi}{2}\cos^2(\frac{\alpha}{2}+\frac{\Delta\alpha}{2}))(2-\cos\alpha\cos\phi-\cos\phi)(3-\cos(\alpha+\Delta\alpha)-\cos\phi-\cos(\alpha+\Delta\alpha)\cos\phi)}}. \tag{S8}$$

Since the denominator is bound, $P_{S\to\perp}$ can only be approach zero, if either $|\cos\frac{\alpha}{2}| \ll 1$, $|1-\cos\phi| \ll 1$, or $|\sin\frac{\Delta\alpha}{2}| \ll 1$. The first condition is essentially equivalent to $\alpha \approx \pi$ and the second condition corresponds to the stop bands (cf. Fig. S4). Both result in a steady state with vanishing magnetization[7], so that the only practical way to avoid the population of the perpendicular transient eigenstates is to fulfill the third condition, i.e. small $\Delta\alpha$. Note that the constraints for the last factor in Eq. (S8) to vanish requires at least one of the three above mentioned to be fulfilled. Therefore, we can neglect this factor here.

For variations of $\phi$, we similarly find the conditions $|\sin\alpha| \ll 1$, $|\sin\phi| \ll 1$, $|\sin(\Delta\phi + 2\phi)| \ll 1$ and $|\sin\frac{\Delta\phi}{2}| \ll 1$ for a vanishing population of the perpendicular transient eigenstate. The first two conditions result in vanishing signal and the third condition describes merely a symmetric oscillation, which has essentially no effect. Consequently, the only practical way to avoid a population of the perpendicular transient eigenstate is a small $\Delta\phi$.

## References


[1] Peter Schmitt, Mark A Griswold, Peter M Jakob, Markus Kotas, Vikas Gulani, Michael Flentje, and Axel Haase. Inversion recovery TrueFISP: quantification of T1, T2, and spin density. *Magn. Reson. Med.*, 51(4):661–667, 2004.

[2] Carl Ganter. Off-resonance effects in the transient response of SSFP sequences. *Magn. Reson. Med.*, 52(2):368–375, 2004.

[3] Jakob Assländer, Steffen J. Glaser, and Jürgen Hennig. Pseudo Steady-State Free Precession for MR-Fingerprinting. *Magn. Reson. Med.*, 77(3):1151–1161, mar 2017.

[4] Klaus Scheffler and Jürgen Hennig. Is TrueFISP a gradient-echo or a spin-echo sequence? *Magn. Reson. Med.*, 49(2):395–397, feb 2003.

[5] Dan Ma, Vikas Gulani, Nicole Seiberlich, Kecheng Liu, Jeffrey L. Sunshine, Jeffrey L. Duerk, and Mark A. Griswold. Magnetic resonance fingerprinting. *Nature*, 495(7440):187–192, 2013.

[6] Sean C L Deoni, Brian K. Rutt, and Terry M. Peters. Rapid combined T1 and T2 mapping using gradient recalled acquisition in the steady state. *Magn. Reson. Med.*, 49(3):515–526, 2003.

[7] H. Carr. Steady-State Free Precession in Nuclear Magnetic Resonance. *Phys. Rev.*, 112(5):1693–1701, 1958.
